# Supplementary material for: Exploring the Danmaku Content Moderation on Video-Sharing Platforms: Existing Limitations, Challenges, and Design Opportunities
Source: arXiv:2411.04529 source file (2024-11-07)
Supplement: Supplementary file 1 [file 06-appendix.tex]

\section{Appendix}

\subsection{Probes List}

\begin{enumerate}
            \item 
        \end{enumerate}

\begin{itemize}
    \item Personal-Control Moderation
        \begin{enumerate}
            \item Content Filtering: Automatically or manually allows users to filter or block specific types or sources of danmaku.
            \item Binary Toggle: Manually enables users to turn danmaku filtering on or off.
            \item Keywords Filtering: Manually allows users to customize danmaku display rules, such as blocking specific users or keywords.
            \item Intelligent Filtering: An automated feature that identifies and filters improper danmaku using preset rules and algorithms.
        \end{enumerate}
    \item Reactive Moderation
        \begin{enumerate}
            \item User Reporting: A semi-automated feature for users to report inappropriate or offensive danmaku for platform review.
            \end{enumerate}
    \item Distributed Moderation
        \begin{enumerate}
            \item Danmaku Voting: A community-driven process where users participate in the moderation through voting.
            \end{enumerate}
    
    \item Community Moderation
    \begin{enumerate}
            \item Community Rules: Automatically enforced rules set by the community to moderate content.
            \end{enumerate}
\end{itemize}
\label{probes_list}

\newpage

\subsection{Design Outputs}
\input{table/designexamples}
